# Supplementary material for: Overcoming Barriers to Computational Reproducibility
Source: arXiv:2602.03863 ancillary file (2026-01-27)
Supplement: Supplementary file 1 [file illustrations_supplement.pdf]

Supplementary Material to the Article:

# Overcoming Barriers to Computational Reproducibility

Roman Hornung<sup>1,2</sup>, László Németh<sup>\*3,4</sup>, Oleksandr Zadorozhnyi<sup>5</sup>, Theresa Ullmann<sup>6</sup>, Michael Kammer<sup>6,7</sup>, Rebecca Killick<sup>8,9</sup>, Christopher J. Paciorek<sup>10</sup>, Julien Chiquet<sup>11</sup>, Moritz Herrmann<sup>2,12</sup>, Lucija Batinović<sup>13,14</sup>, Rickard Carlsson<sup>14</sup>, Pierre Neuvial<sup>15</sup>, Boris Hejblum<sup>16</sup>, Julia Wrobel<sup>17</sup>, Anne-Laure Boulesteix<sup>12,2</sup>, and Karsten Tabelow<sup>3</sup>

<sup>1</sup>Department of Statistics, Ludwig-Maximilians-Universität (LMU), Munich, Germany

<sup>2</sup>Munich Center for Machine Learning (MCML), Munich, Germany

<sup>3</sup>Weierstrass Institute for Applied Analysis and Stochastics, Berlin, Germany

<sup>4</sup>Max Planck Institute for Demographic Research, Rostock, Germany

<sup>5</sup>Department of Computer Science, TUM School of Computation, Information and Technology, Technical University of Munich, Munich, Germany

<sup>6</sup>Institute of Clinical Biometrics, Center for Medical Data Science, Medical University of Vienna, Vienna, Austria

<sup>7</sup>Division of Nephrology and Dialysis, Department of Medicine III, Medical University of Vienna, Vienna, Austria

<sup>8</sup>School of Mathematical Sciences, Lancaster University, Lancaster, United Kingdom

<sup>9</sup>School of Mathematical and Statistical Sciences, Clemson University, Clemson, USA

<sup>10</sup>Department of Statistics, University of California, Berkeley, USA

<sup>11</sup>UMR MIA Paris-Saclay, INRAE, AgroParisTech, Université Paris-Saclay, Palaiseau, France

<sup>12</sup>Institute for Medical Information Processing, Biometry, and Epidemiology, Faculty of Medicine, Ludwig-Maximilians-Universität (LMU), Munich, Germany

<sup>13</sup>Department of Behavioural Sciences and Learning, Linköping University, Linköping, Sweden

<sup>14</sup>Department of Psychology, Linnaeus University, Växjö, Sweden

<sup>15</sup>Institut de Mathématiques de Toulouse (IMT), CNRS, Université de Toulouse, Toulouse, France

<sup>16</sup>SISTM, U1219 Bordeaux Population Health, Université de Bordeaux / INSERM / Inria, Bordeaux, France

<sup>17</sup>Department of Biostatistics and Bioinformatics, Emory University, Atlanta, USA

---

\*Corresponding author: nemeth@wias-berlin.de

## Contents

|          |                                                                             |          |
|----------|-----------------------------------------------------------------------------|----------|
| <b>A</b> | <b>Illustrative example of the code and data supplement and README file</b> | <b>3</b> |
| A.1      | Directory structure (illustrative) . . . . .                                | 3        |
| A.2      | Schematic example of a README file . . . . .                                | 3        |
| <b>B</b> | <b>Illustrative examples for reproducible parallel analyses</b>             | <b>6</b> |
| B.1      | Example in R using the <code>future</code> ecosystem . . . . .              | 6        |
| B.2      | Example in Python using NumPy's SeedSequence-based RNG . . . . .            | 9        |

## A Illustrative example of the code and data supplement and README file

### A.1 Directory structure (illustrative)

```
code_and_data/  
|-- data/  
|   |-- (input data files, e.g., survey.csv, cohort.parquet, and the codebook)  
|-- code/  
|   |-- 00_functions.R  
|   |-- 01_simulation.R  
|   |-- 02_real_data_analysis.R  
|   |-- 03_evaluation.R  
|-- results/  
|   |-- intermediate_results/  
|       |-- sim_results.Rda  
|       |-- real_results.Rda  
|   |-- figures/  
|       |-- figure1.png  
|       |-- figure2.pdf  
|   |-- tables/  
|       |-- table1.csv  
|       |-- table2.tex  
|-- README.txt
```

### A.2 Schematic example of a README file

**Title:** Code and data supplement for <Article Title>

**Corresponding author:** <Name, Email>

**Purpose** This supplement reproduces all figures and tables reported in the article and supplement. It provides both (i) scripts that generate the raw analysis outputs (`results/intermediate_results/*.Rda`) and (ii) scripts that transform these intermediate outputs into the final figures and tables.

#### Contents

- **data/** – Input data required for the real-data analysis (file formats may include `.csv`, `.parquet`, etc.). If data cannot be shared, see notes below.
- **code/**
  - `00_functions.R` – Helper functions used across scripts.
  - `01_simulation.R` – Generates simulated results saved to `results/intermediate_results/sim_results.Rda`.

- `02_real_data_analysis.R` – Runs analysis on the real dataset and saves outputs to `results/intermediate_results/real_results.Rda`.
- `03_evaluation.R` – Produces all final figures and tables from the intermediate results.
- **results/**
  - **intermediate\_results/** – Raw outputs of the analysis (R data objects, `*.Rda`).
  - **figures/** – Final figures as referenced in the article.
  - **tables/** – Final tables as `.csv/.tex` as referenced in the article.
- **README.txt** – This file.

## Reproduction instructions

### Option A: Full regeneration (including raw analysis outputs).

1. Ensure the working directory to be at the `code_and_data/` root and that all paths in the scripts are relative (no absolute paths).
2. Execute, in order:

```
code/01_simulation.R
code/02_real_data_analysis.R
code/03_evaluation.R
```

3. Final outputs are written to `results/figures/` and `results/tables/`.

### Option B: Fast reproduction of final outputs (using provided intermediate results).

1. Skip `01_simulation.R` and `02_real_data_analysis.R`.
2. Run:

```
code/03_evaluation.R
```

3. This recreates all figures and tables from the available intermediate results.

## Mapping of scripts to reported outputs

- `code/03_evaluation.R` produces:
  - Figure 1: `results/figures/figure1.png`
  - Figure 2: `results/figures/figure2.pdf`
  - Table 1: `results/tables/table1.csv`
  - Table 2: `results/tables/table2.tex`

**Software environment (recorded via `sessionInfo()`)** Paste or regenerate the exact session info used to produce the results. An illustrative (schematic) example:

```
R version 4.2.2 Patched (2022-11-10 r83330)
Platform: x86_64-pc-linux-gnu (64-bit)
Running under: Debian GNU/Linux 12 (bookworm)
```

```
Matrix products: default
BLAS/LAPACK: Accelerate framework
```

attached base packages:

```
[1] stats graphics grDevices utils datasets methods base
```

other attached packages:

```
[1] ggplot2_3.4.4 dplyr_1.1.3
```

loaded via a namespace (and not attached):

```
[1] tibble_3.2.1 tidyr_1.3.0 readr_2.1.4
```

**Data availability notes** If legal/ethical constraints prevent sharing full datasets, provide either (i) instructions for controlled access, or (ii) synthetic data that mimic the structure and essential properties of the real data in combination with the results obtained using this synthetic data (see the main paper for more details on this).

## B Illustrative examples for reproducible parallel analyses

This section provides two minimal, fully reproducible code examples—one in R and one in Python—that illustrate how to

- run a simple simulation in parallel,
- associate each replication with its own deterministic random number stream, and
- later rerun an individual replication (interactively) to inspect intermediate calculations.

In both examples, we estimate the mean of normally distributed data in several independent replications. The examples are intentionally simple so that they can serve as templates for more complex analyses.

### B.1 Example in R using the future ecosystem

The following R code uses the `future` and `future.apply` packages to run a small simulation in parallel. Each replication has its own deterministic random number stream (controlled via `future.seed`), and we store the RNG state at the start of each replication so that any replication can later be reproduced step by step in a sequential R session.

```
# R example: reproducible parallel simulation with per-replication streams
```

```
# Required packages:
```

```
library(future)
```

```
library(future.apply)
```

```
# Use a parallel plan with a fixed number of workers (e.g., 5)
```

```
plan(multisession, workers = 5)
```

```
n_rep      <- 8      # number of replications
```

```
n_per_rep  <- 100    # sample size per replication
```

```
root_seed  <- 123    # arbitrary but fixed root seed
```

```
# One replication: draw  $N(0, 1)$  data and compute the sample mean.
```

```
# We also record the RNG state at the start of this replication.
```

```
simulate_one <- function(rep_id) {
```

```
  rng_state_start <- .Random.seed
```

```
  x <- rnorm(n_per_rep, mean = 0, sd = 1)
```

```
  m <- mean(x)
```

```
  list(
```

```
    rep_id = rep_id,
```

```
    mean   = m,
```

```

    rng_state = rng_state_start
  )
}

# Run the simulation in (potentially) parallel.
# 'future.seed = TRUE' asks the future framework to create
# parallel-safe, deterministic random number streams.
set.seed(root_seed)
results <- future_lapply(
  X          = seq_len(n_rep),
  FUN        = simulate_one,
  future.seed = TRUE
)

# Extract the means from all replications
sapply(results, function(x) x$mean)

# Reset to sequential execution and shut down background workers
plan(sequential)

```

The object `results` now contains, for each replication,

- the replication index (`rep_id`),
- the estimated mean (`mean`), and
- the RNG state at the start of that replication (`rng_state`).

To interactively reproduce a single replication (for example, replication 3) and step through the code line by line, one can use the stored RNG state as follows:

```

# Choose the replication to inspect
k <- 3

# Restore the RNG state for replication k
assign(".Random.seed", results[[k]]$rng_state, envir = .GlobalEnv)

# Now rerun the body of simulate_one(k) interactively:
x <- rnorm(n_per_rep, mean = 0, sd = 1)
mean(x) # this will be identical to results[[k]]$mean

```

In more complex analyses, the function `simulate_one()` would contain additional computation steps. The same pattern applies: by restoring the stored RNG state and then executing the function body line by line, individual replications can be examined in detail while remaining numerically reproducible.

**Software environment (R).** The complete software environment used to generate the R example is documented below to support long-term reproducibility.

R version 4.4.0 (2024-04-24 ucrt)

Platform: x86\_64-w64-mingw32/x64

Running under: Windows 11 x64 (build 26100)

Matrix products: default

Random number generation:

RNG: L'Ecuyer-CMRG

Normal: Inversion

Sample: Rejection

locale:

[1] LC\_COLLATE=German\_Germany.utf8 LC\_CTYPE=German\_Germany.utf8

[3] LC\_MONETARY=German\_Germany.utf8 LC\_NUMERIC=C

[5] LC\_TIME=German\_Germany.utf8

time zone: Europe/Berlin

tzcode source: internal

attached base packages:

[1] stats graphics grDevices utils datasets methods base

other attached packages:

[1] future.apply\_1.11.2 future\_1.34.0

loaded via a namespace (and not attached):

[1] digest\_0.6.35 RColorBrewer\_1.1-3 R6\_2.6.1 codetools\_0.2-20

[5] farver\_2.1.2 glue\_1.7.0 parallel\_4.4.0 lifecycle\_1.0.4

[9] cli\_3.6.2 scales\_1.4.0 parallelly\_1.38.0 compiler\_4.4.0

[13] globals\_0.16.3 rstudioapi\_0.16.0 tools\_4.4.0 listenv\_0.9.1

[17] rlang\_1.1.3

## B.2 Example in Python using NumPy's SeedSequence-based RNG

The following Python code uses NumPy's random number generation, which is based on `SeedSequence`. Each replication receives its own deterministic random number generator, created from a combination of a global root seed and the replication index. The simulation is run in parallel using `concurrent.futures`.

```
# Python example: reproducible parallel simulation with per-replication streams
```

```
import numpy as np
from concurrent.futures import ProcessPoolExecutor

n_rep      = 8      # number of replications
n_per_rep  = 100     # sample size per replication
root_seed  = 12345   # arbitrary but fixed root seed

def simulate_one(rep_id, root_seed, n_per_rep):
    # Create a per-replication RNG using SeedSequence under the hood.
    # The list [rep_id, root_seed] defines a unique, deterministic stream.
    rng = np.random.default_rng([rep_id, root_seed])
    x = rng.normal(loc=0.0, scale=1.0, size=n_per_rep)
    m = x.mean()
    return {"rep_id": rep_id, "mean": float(m)}

def main():
    # Run the simulation in parallel with a fixed number of workers (e.g., 5)
    with ProcessPoolExecutor(max_workers=5) as ex:
        futures = [
            ex.submit(simulate_one, rep_id, root_seed, n_per_rep)
            for rep_id in range(n_rep)
        ]
        results = [f.result() for f in futures]

    # Extract the means from all replications
    [res["mean"] for res in results]

if __name__ == '__main__':
    main()
```

Here, each replication `rep_id` uses its own generator `default_rng([rep_id, root_seed])`, which ensures a deterministic and parallel-safe random number stream for that replication.

To reproduce one specific replication (for example, `rep_id = 3`) in an interactive Python session and inspect intermediate objects, one can proceed as follows:

```
# Reproduce a single replication (rep_id = 3) interactively
```

```

rep_id = 3
rng = np.random.default_rng([rep_id, root_seed])

x = rng.normal(loc=0.0, scale=1.0, size=n_per_rep)
x.mean() # this will match the stored mean for rep_id = 3

```

As with the R example, in more complex simulations the function `simulate_one` would contain additional steps. The key idea is that the combination of `root_seed` and `rep_id` uniquely defines the random number stream, so that any given replication can be recomputed exactly and investigated in detail.

**Software environment (Python).** The complete software environment used to generate the Python example is documented below to support long-term reproducibility.

```

-----
numpy                2.3.3
session_info         v1.0.1
-----
Python 3.14.0 (tags/v3.14.0:ebf955d, Oct  7 2025, 10:15:03) [MSC v.1944 64 bit (AMD64)]
Windows-11-10.0.26200-SP0
-----
Session information updated at 2025-12-04 13:01

```
